# Supplementary material for: Are multi-quasiparticle interactions important in molecular ionization?
Source: arXiv:2009.02401 ancillary file (2020-12-01)
Supplement: Supplementary file 1 [file SI.pdf]

# Supporting Information for "Are multi-quasiparticle interactions important in molecular ionization?"


Carlos Mejuto-Zaera,[†] Guorong Weng,[‡] Mariya Romanova,[‡] Stephen J. Cotton,[¶] K. Birgitta Whaley,[†] Norm M. Tubman,[¶] and Vojtěch Vlček[*,‡]

*†University of California, Berkeley, California 94720, United States*

*‡University of California, Santa Barbara, California 93106, United States*

*¶Quantum Artificial Intelligence Lab. (QuAIL), Exploration Technology Directorate, NASA Ames Research Center, Moffett Field, CA 94035, USA*

*§KBR, 601 Jefferson St., Houston, TX 77002*

E-mail: vlcek@ucsb.edu

December 1, 2020

# Methodological details

## ASCI - Ground State

The idea behind the ASCI algorithm is to find an optimal truncation $\mathcal{T}^N$ of a given size $|\mathcal{T}^N|$ of the full Hilbert space, in order to accurately describe the ground state of a many-body Hamiltonian. ASCI has previously been shown to be able to successfully identify optimal truncations for a wide variety of systems across the fields quantum chemistry and condensed matter physics, including several molecular systems, the uniform electron gas, the two-dimensional square lattice Hubbard model and Hubbard-Anderson impurity models of the sort typically found in dynamical mean-field theory calculations.[1,2] Effectively, we specify as input the size $|\mathcal{T}^N|$ of the truncation that we can afford, i.e., a number of Slater determinants into which the full Hilbert space is truncated, as well as the Hamiltonian of interest $H$ in some single-particle basis. The ASCI algorithm returns the most important $|\mathcal{T}^N|$ many-body Slater determinants for the description of the ground state wave function $|\Psi_0\rangle$ of $H$. We can then project the Hamiltonian $H$ onto that truncation space, and compute the approximate ground state wave function $|\psi_0\rangle$ and the approximate ground state energy $E_0$.

The key element in the ASCI algorithm is the introduction of a ranking criterion, which given two determinants allows to estimate which one is more important for the ground state wave function. Using this ranking criterion, the identification of the optimal truncation space is performed iteratively, exploring regions of the Hilbert space connected through $H$ to a given reference truncation $\mathcal{T}^N$. After the exploration staga, all new determinants together with the determinants in $\mathcal{T}^N$ are ranked. Finally, we build a new truncation $\mathcal{T}'^N$ by keeping only the $|\mathcal{T}^N|$ most important determinants in the ranking. The Hamiltonian is then diagonalized in the new truncation $\mathcal{T}'^N$, getting new ground state energy and wave

function estimates. The process is repeated until the ground state energy $E_0$ converges to the desired accuracy.

The ASCI algorithm performs best for systems with (a) a high Hamiltonian connectivity, which accelerates the search, and (b) a true ground state that is well described by a few states in some one-body basis. Both of these conditions are usually fulfilled in molecular systems. The dense two-body term in the molecular Hamiltonian in typical quantum chemistry basis-sets accounts for point (a). An optimal one-body basis, in the sense described by condition (b), can be found by introducing rotation to natural orbitals through the ASCI calculation. These rotations are usually performed in the first few iterations and are crucial to achieving a compact truncation, i.e. an accurate truncation that is a small as possible. For more detailed on the ASCI algorithm, see.[1,3,4]

## ASCI - Green's Function

Having determined the optimal truncation $\mathcal{T}^N$ and the corresponding ground state wave function $|\psi_0\rangle$ and energy $E_0$, one can compute the Green's function by evaluating eq 1. In[5] we showed that the fast convergence of the ground state energy with the size $\left|\mathcal{T}^N\right|$ of $\mathcal{T}^N$ is inherited by the Green's function, which also converges rapidly with the number of determinants in the truncated space. The particle and hole components of the Green's function are computed separately using the Lanczos algorithm.[6,7] The Green's function evaluation can be conceptually split into two steps: identifying a truncated basis in the particle (hole) sector and evaluation of the ref in that truncated basis.

We want to build the truncated basis in the particle (hole) sector $\mathcal{T}^{N+1}$ ($\mathcal{T}^{N-1}$) on top of the truncated space in the $N$ particle sector $\mathcal{T}^N$, that is returned by ASCI. Unlike in previous studies,[5] where a different basis was built for each Green's function matrix element, here we build a single basis in the particle (hole) sector that is common to all elements of the Green's function. For this, we build a partial basis $\mathcal{T}_i^{N\pm1}$ for each orbital $i$, and then form the total basis as the union of these partial bases, i.e.

$$\mathcal{T}^{N\pm 1} = \cup_i \ \mathcal{T}_i^{N\pm 1}. \tag{1}$$

In order to form $\mathcal{T}_i^{N\pm1}$, we build an initial "naive" truncated space $\mathcal{T}_i^{N+1,0}$ by applying the corresponding creation (annihilation) operator $c_i^\dagger$ ($c_i$) to all determinants in $\mathcal{T}^N$. The union of these naive spaces, which will be at most $p$ times as large as $\mathcal{T}^N$, where $p$ is the number of orbitals, would be enough to compute matrix elements like $\langle\psi_0|c_i H c_j^\dagger|\psi_0\rangle$ within ASCI accuracy. However, the Green's function requires inverting the Hamiltonian and thus more determinants are needed in general. We expand the naive truncations by adding "layers" of single and double excitations of the determinants in $\mathcal{T}_i^{N+1,0}$. If we apply $m$ layers, we add new determinants that are $1, 2, \ldots, m$ single or double excitations away form the determinants in $\mathcal{T}_i^{N+1,0}$. In general, we do not add these layers of excitations on top of all the determinants in a given naive space, but only on top of those generated from determinants in $\mathcal{T}^N$ that possess a ground state wave function coefficient above some threshold. For the computations presented in this work, we choose this threshold to be $10^{-3}$. In[5] we showed that for the typical impurity models found in dynamical mean-field theory calculations on the Hubbard model, two layers of excitations were sufficient to converge the spectral functions along the real frequency axis. In the small molecular examples in this work, one layer was enough. Furthermore, in these layers we add only single excitations and no doubles.

Using only a small number of layers is fundamental, since the size of the truncated spaces increases exponentially with the number of applied layers. To further reduce the size of each $\mathcal{T}_i^{N+1}$ without compromising accuracy, we exploit the active space structure of the orbital space $\{c_i\}$, identifying those orbitals with occupation close to 2 or 0 as inactive, and the rest as active. When adding layers of excitations, we then only consider excitations from and to active orbitals. This can significantly reduce the size of $\mathcal{T}_i^{N+1}$. We consider an orbitals as "active" if it's average occupation in the ground state wave function $\langle n_i\rangle_0$ fufills $10^{-4} \leq \langle n_i\rangle_0 \leq 2 - 10^{-4}$. The natural orbital rotations introduced in the ground state

calculation optimize this active space, since they tend to maximize the number of inactive orbitals.

We note that due to the way in which the naive truncations $\mathcal{T}_i^{N+1}$ ($\mathcal{T}_i^{N-1}$) are built, using the corresponding creation (annihilation) operators, the final truncation spaces for different orbitals will in general be different. In the exact diagonalization limit (the full configuration interaction limit), i.e., when the ASCI truncation $\mathcal{T}^N$ is equal to the full Hilbert space in the $N$ particle sector, then all the partial truncations $\mathcal{T}_i^{N+1}$ for all orbitals become equal and identical to the full Hilbert space in the $(N+1)$ particle sector. It is then unnecessary to build more than one of the "partial" truncations in this limit. Moreover, it is only necessary to apply one layer of excitations on top of the naive truncation space to recover the full Hilbert space.

For a given orbital $i$, the sizes of the particle and hole truncations, $\left|\mathcal{T}_i^{N+1}\right|$ and $\left|\mathcal{T}_i^{N-1}\right|$, can be very different. In particular, an orbital that is full, or mostly full, in the ground state will have a much smaller $\left|\mathcal{T}_i^{N+1}\right|$ than $\left|\mathcal{T}_i^{N-1}\right|$. This is because most important determinants in the ground state wave function will likely have that orbital occupied, such that when applying $c_i^\dagger$ these determinants do not contribute to $\mathcal{T}_i^{N+1}$. Conversely, an orbital that is empty or mostly empty will have a much smaller $\left|\mathcal{T}_i^{N-1}\right|$ than $\left|\mathcal{T}_i^{N+1}\right|$. For partially occupied orbitals, i.e. orbitals with an average occupation in the ground state $\langle n_i \rangle_0$ close to 1, both spaces will be of comparable size. As a result of these differences, for the small molecular systems studied in this work and also when using a large basis set, $\left|\mathcal{T}_i^{N+1}\right|$ will be much larger than $\left|\mathcal{T}_i^{N-1}\right|$, because there are far more orbitals than electrons. Since the systems studied here are not particularly strongly correlated, there are at most of the order of 30-40 active orbitals in the ground state of any of the five systems. Of those, only $n_{el}/2$ spatial orbitals are substantially occupied, where $n_{el}$ is the number of electrons. Consequently, the full hole truncated bases $\mathcal{T}^{N-1}$ built as explained above only have relevant contributions of $n_{el}/2$ orbitals (in this work between 5-7), while $\mathcal{T}^{N+1}$ has relevant contributions from all unoccupied virtual orbitals. The number of the latter in an augmented quadruple zeta basis

is of the order of 100, so $\mathcal{T}^{N+1}$ will be about two orders of magnitude larger than $\mathcal{T}^{N-1}$. This makes computing the particle component of the Green's function much more computationally demanding than the hole component. In this work we have concentrated on the negative frequency part of the spectral function $A(\omega)$. This simplifies the calculations, since, for any many-body system, the particle component of the ground state Green's function has all diagonal elements equal to zero for $\omega < 0$. Thus, to compute the spectral function $A(\omega)$, we do not need the particle Green's function.

Once the full truncated basis $\mathcal{T}^{N+1}$ (or $\mathcal{T}^{N-1}$ for the hole component) has been determined, we evaluate the particle component of eq 1 using the Lanczos algorithm.[6,7] In our previous work[5] we used the simple one-band Lanczos method[6] to compute all elements of the Green's function one at a time. This strategy, amenable to trivial parallelization, is ideal if one is interested in the different elements of the Green's function independently, for example when one only wants to determine the spectral function $A(\omega) = -\frac{1}{\pi}\Im G(\omega)$. In these cases, it is sufficient to find for each Green's function element the optimal truncations $\mathcal{T}^{N\pm1}$, which as noted above will be in general different for each element $G(\omega)^{p}_{i,j}$. This can become an issue when using a truncated Hilbert space, as is the case in ASCI, for systems in which different orbitals show a significant degree of coupling. This was the case for the molecules studied in this work, since as discussed in the main paper the orbital resolved spectral function $A(\omega)_i = -\frac{1}{\pi}\Im\left[G(\omega)_{i,i}\right]$ for orbital $i$ showed satellites resonant with the main quasiparticle energies of another orbital $j$. In order to capture these features accurately, we used a common basis for all elements of the Green's function, by building the union of the partial truncations corresponding to each orbital. Instead of computing each Green's function element in parallel, we employed the band Lanczos algorithm[7] to determine all at the same time, reducing the computational time significantly. Using band Lanczos, and a common truncation basis for all Green's function elements, ensured an accurate description of inter-orbital resonant features with modest sized truncations. The price for the time saving using band Lanczos is in memory, since it requires storing more vectors simultaneously than

the two that are formally needed in the one-band formulation. Thanks to the compactness of the $\mathcal{T}^{N\pm1}$ spaces, we could afford the memory demands, since each vector had at most ~7 million elements (in the case of $N_2$ in the aug-cc-pvqz basis). The band Lanczos method has received relative little attention in the many-body literature, and thus we briefly summarize the main idea and properties of the method here, following the presentation of.[7]

The band Lanczos method is a natural generalization of the common Lanczos algorithm, which uses several linearly independent initial vectors instead of only one. In $n$ band Lanczos, one starts thus with an orthonormal set of vectors $\left\{\tilde{\psi}_i\right\}_{i=1}^{n}$.[1] Then, one builds a Krylov space formed by actions of the Hamiltonian $H$ on this starting set. In each iteration, one acts with $H$ on a vector in the Krylov space, and makes it orthogonal to the previous ones using a recursion relation. Unlike in one-band Lanczos, where the recursion relation involves only three vectors at a time, this band Lanczos verison involves $2n + 1$ vectors. Thus, one needs to store in memory the last $2n$ vectors in the Krylov space, resulting in the higher memory demand of the band Lanczos method compared to simple Lanczos. During the iterative process, the Hamiltonian matrix in the Krylov basis is evaluated. While in one-band Lanczos the Hamiltonian is tridiagonal in the Krylov basis, in $n$ band Lanczos the Hamiltonian is band-diagonal, with $n$ non-vanishing upper- and lower-diagonals. After $j$ iterations, during which one has gone over the span of each of the original $\left\{\tilde{\psi}_i\right\}_{i=1}^{n}$ vectors $J = \lfloor \frac{j}{n} \rfloor$ times, one has formed the Hamiltonian $H^{(j)}$. Similarly to one-band Lanczos, this Krylov Hamiltonian fulfills the following relations with respect to the set $\left\{\tilde{\psi}_i\right\}_{i=1}^{n}$:[7]

[1]For the Green's function calculation, e.g. in the particle sector, $n$ equals the number of orbitals and the starting vectors are orthonormalized linear combinations of $\left\{c_i^\dagger \left|\psi_0\right\rangle\right\}_{i=1}^{n}$. This orthonormalization is performed by QR factorization.

$$\left(H^{(j)}\right)^k |\widetilde{\psi}_i\rangle = \quad H^k |\widetilde{\psi}_i\rangle\,, \quad \text{for } 1 \leq i \leq n, \tag{2}$$

$$\text{for } 0 \leq k \leq J-1$$

$$\langle\widetilde{\psi}_i| \left(H^{(j)}\right)^k |\widetilde{\psi}_h\rangle = \quad \langle\widetilde{\psi}_i|H^k|\widetilde{\psi}_h\rangle\,, \quad \text{for } 1 \leq i, h \leq n, \tag{3}$$

$$\text{for } 0 \leq k \leq 2J-1,\ k \text{ odd}$$

$$\text{for } 0 \leq k \leq 2J-2,\ k \text{ even.}$$

Thus the first $2J-2$ powers of the Krylov Hamiltonian have the exact same matrix elements with the initial set $\left\{\tilde{\psi}_i\right\}_{i=1}^{n}$ as does the full Hamiltonian. This equivalence of Hamiltonian powers provides a fast convergence of the Green's function with the number of Lanczos iterations, which can also be understood in terms of the moments of the spectral function.[6] It should be noted that for the same number of iterations $j$, the one-band Lanczos method equates more expectation values than $n$ band Lanczos, since $J = \lfloor \frac{j}{n} \rfloor$. If necessary, the same number of powers can be recovered in the band Lanczos method by increasing the number of iteration by a factor linear with the number of orbitals, although this is rarely necessary. For the calculations presented in this work, due to the weakly correlated ground state structure of the closed-shell molecules considered here, we only need to consider the $n_{el}/2$ lowest orbitals when determining the Green's function. Effectively, we only computed an at most $7 \times 7$ block of the full Green's function matrix. Thus, a standard number of 4000 band Lanczos iterations was sufficient to obtain reliable Green's functions.

## ASCI - Simulation Parameters

For the small closed-shell molecular systems studied in this work, we performed an ASCI ground state calculation with $\left|\mathcal{T}^N\right| = 5 \cdot 10^5$ determinants using cc-pvXz and aug-cc-pvXz basis sets, where X = D,T,Q. For $CH_4$, we were not able to use the aug-cc-pvQz basis set, so we only report results for the other five basis sets. To determine the spectral function

$A(\omega)$ for $\omega < 0$, we subsequently constructed the hole truncated space $\mathcal{T}^{N-1}$. We proceed as described above, using one layer of single excitations and a frequency spacing of 0.05 eV.

## ASCI - $A(\omega)$ convergence with the truncation space size

Fig. S1 shows the hole component of the spectral function $A(\omega)$ for select systems and different basis sets. We see that the main quasiparticle energies show excellent convergence with the number of states, with no appreciable change over a wide range of values of $\left|\mathcal{T}^{N}\right|$. While different systems and basis sets show slightly different convergence behavior, in general the position of the QPEs could be always be converged within 0.15 eV, in the sense that results shown in the main paper would change by no more than 0.15 eV on increasing the truncation space size by a factor of 5. The satellite features also show a satisfactory qualitative convergence with respect to the size of the target space.

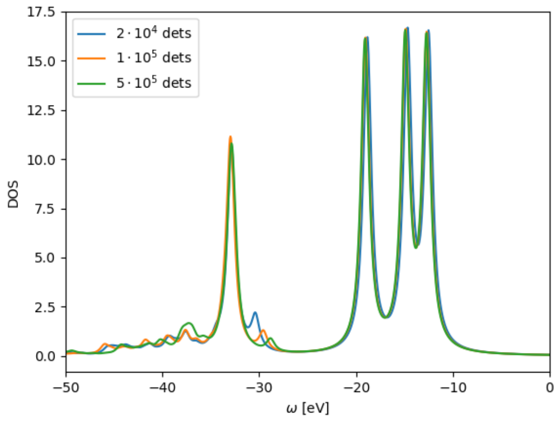


(a) $H_2O$.

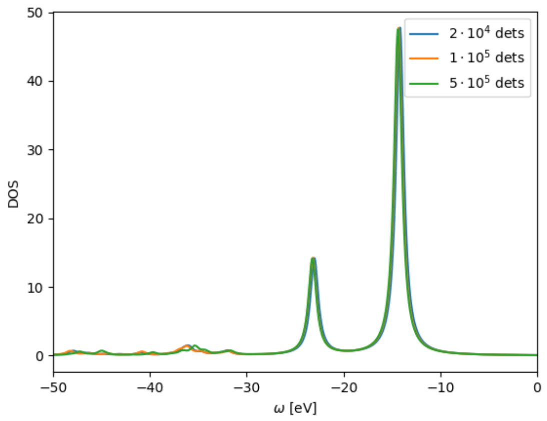


(b) $CH_4$.

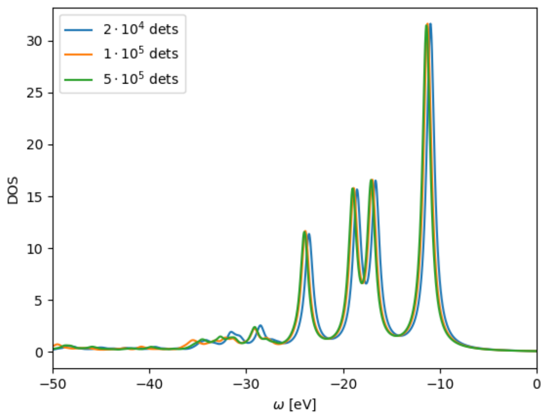


(c) $C_2H_2$.

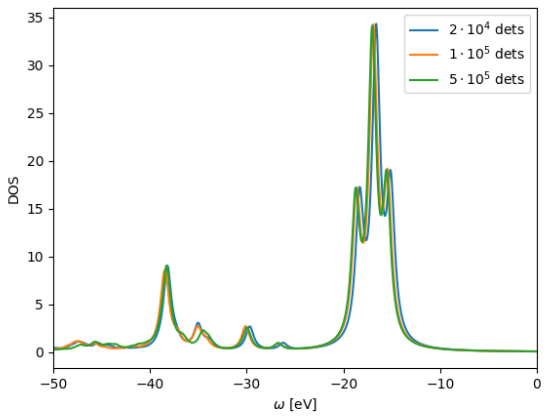


(d) $N_2$.

Figure S1: Hole component of the spectral function for the occupied orbitals of the molecules studied with aug-cc-pvqz basis sets and different ASCI truncations. We use a broadening factor of 0.5 eV.

## ASCI - $A(\omega)$ convergence with basis set

Fig. S2 shows the convergence of the hole component of spectral function as a function of the basis set for all five molecular systems presented in the main paper. We extrapolated the quasiparticle energies to the complete basis set limit following the prescription in.[8] Here as well, the qualitative convergence of the satellite features is satisfactory.

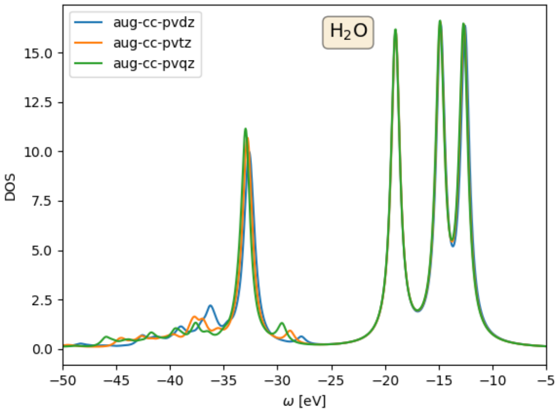


(a) $H_2O$.

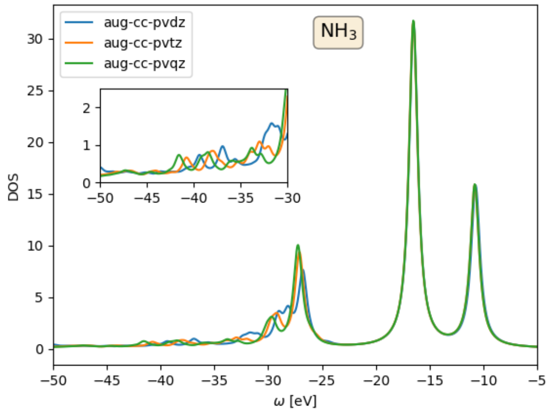


(b) $NH_3$.

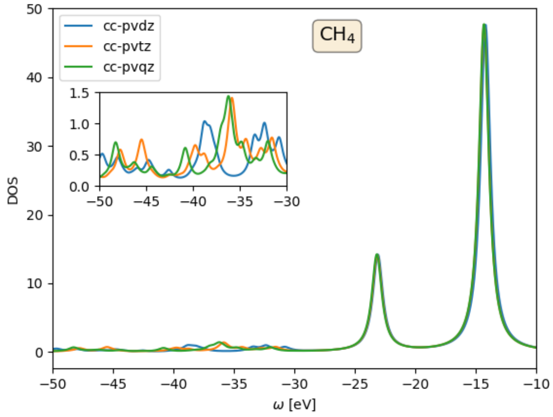


(c) $CH_4$.

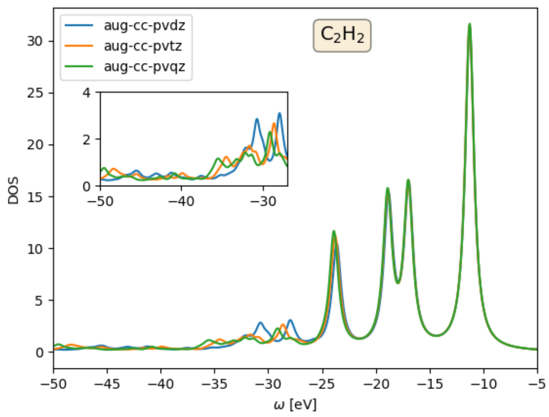


(d) $C_2H_2$.

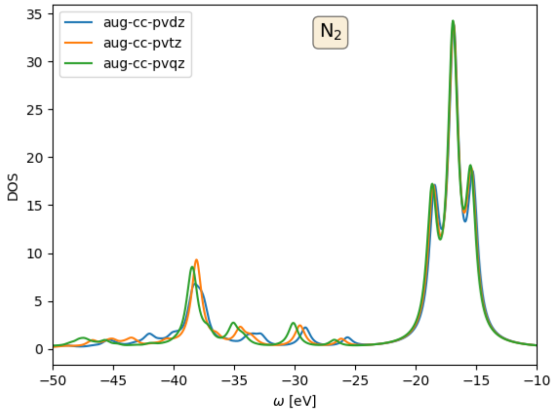


(e) $N_2$.

Figure S2: Hole component of the spectral function for the molecules studied with different augmented, correlation consistent basis sets and an ASCI truncation of $10^5$ determinants. We use a broadening factor of $\sim 0.5$ eV.

## ASCI - quasiparticle Energies

In Tab. S1 we report the quasiparticle energies for all valence orbitals and all molecules studied in the main paper with different basis sets. We also show the results with basis set extrapolation using the prescription in.[8] These results are computed with ASCI using a truncated space of $5 \cdot 10^5$ states, using a broadening of 0.50 eV. For the lowest lying valence orbital of $N_2$ we report only the position of the highest peak. The apparent jumps in the QP energies for this lowest lying orbital in $N_2$ when going from double to triple zeta basis are due to weight redistribution among these peaks, which changes the identity of the largest contribution. As discussed above, the quasiparticle energy convergence with the size of the truncated space appears to be reached within a confidence interval of $\pm 0.15$ eV. The extrapolated quasiparticle energies from the augmented and non-augmented basis sets are in good agreement with each other.

We note that, similar to the inter-orbital resonances in the $GW\Gamma$ self-energies discussed in the main paper, the orbital resolved ASCI spectral functions also present resonances. Fig. S3 shows the orbital resolved spectral functions $A(\omega)_i$ for all molecules. With the exception of $CH_4$, all show small resonant peaks between the orbital furthest from the HOMO and at least one of the other orbitals. The $A(\omega)_i$ for the orbital furthest from the HOMO is emphasized with an arrow. However, this resonances appear in the ASCI spectral functions due to the mixed character of the natural orbital basis in which they are computed. Rotating the ASCI Green's functions to the HF basis eliminates the resonances. This leaves the question whether the resonances observed in the $GW\Gamma$ self-energies have a similar "artificial" origin, i.e. related to a physically inconsequential orbital basis rotation. While all MBPT calculations where performed in the HF basis, which would thus suggest a different origin, we must consider the fact that using a space grid instead of a Gaussian basis set (see below) may induce some degree of orbital mixing, akin to the one obtained from natural orbital rotations. Thus, it is unclear whether the self-energy resonances have an actual physical, or in contrast purely computational origin.

**Table S1: QPE's of the valence orbitals for $H_2O$, $NH_3$, $CH_4$, $C_2H_2$ and $N_2$ in different basis sets. The QPE's correspond to the maxima of the negative part of the imaginary hole component Green's function for the valence orbitals. These were computed with ASCI using $10^5$ states.**

| orbital | cc-pvdz | cc-pvtz | cc-pvqz | cc-extrapol. | aug-cc-pvdz | aug-cc-pvtz | aug-cc-pvqz | aug-extrapol. |
|---|---|---|---|---|---|---|---|---|
| $H_2O$-1 | -32.57 | -32.67 | -32.87 | -33.05 | -32.57 | -32.72 | -32.87 | -32.99 |
| $H_2O$-2 | -18.51 | -18.86 | -19.01 | -19.15 | -19.01 | -19.01 | -19.06 | -19.10 |
| $H_2O$-3 | -14.26 | -14.71 | -14.86 | -14.95 | -14.81 | -14.91 | -14.91 | -14.90 |
| $H_2O$-4 | -11.96 | -12.46 | -12.66 | -12.79 | -12.56 | -12.66 | -12.71 | -12.75 |
| $NH_3$-1 | -27.51 | -27.31 | -27.36 | -27.48 | -27.36 | -27.31 | -27.31 | -27.36 |
| $NH_3$-2 | -16.21 | -16.46 | -16.56 | -16.61 | -16.51 | -16.56 | -16.51 | -16.51 |
| $NH_3$-3 | -16.21 | -16.46 | -16.56 | -16.63 | -16.51 | -16.56 | -16.51 | -16.51 |
| $NH_3$-4 | -10.31 | -10.71 | -10.86 | -10.95 | -10.76 | -10.86 | -10.81 | -10.81 |
| $CH_4$-1 | -23.06 | -23.16 | -23.21 | -23.25 | -23.06 | -23.16 | | |
| $CH_4$-2 | -14.21 | -14.36 | -14.36 | -14.35 | -14.26 | -14.36 | | |
| $CH_4$-3 | -14.21 | -14.36 | -14.36 | -14.35 | -14.26 | -14.36 | | |
| $CH_4$-4 | -14.21 | -14.36 | -14.36 | -14.35 | -14.26 | -14.36 | | |
| $C_2H_2$-1 | -23.66 | -23.81 | -24.01 | -24.14 | -23.66 | -23.86 | -24.01 | -24.13 |
| $C_2H_2$-2 | -18.71 | -18.91 | -19.01 | -19.08 | -18.86 | -18.96 | -19.01 | -19.05 |
| $C_2H_2$-3 | -16.86 | -17.01 | -17.11 | -17.18 | -16.96 | -17.06 | -17.11 | -17.15 |
| $C_2H_2$-4 | -11.21 | -11.31 | -11.41 | -11.48 | -11.31 | -11.36 | -11.41 | -11.45 |
| $C_2H_2$-5 | -11.21 | -11.31 | -11.41 | -11.48 | -11.31 | -11.36 | -11.41 | -11.45 |
| $N_2$-1 | -38.12 | -38.02 | -38.27 | -38.47 | -38.12 | -37.97 | -38.27 | -38.56 |
| $N_2$-2 | -18.26 | -18.56 | -18.71 | -18.82 | -18.46 | -18.61 | -18.76 | -18.88 |
| $N_2$-3 | -16.66 | -16.91 | -17.01 | -17.08 | -16.86 | -16.96 | -17.01 | -17.05 |
| $N_2$-4 | -16.66 | -16.91 | -17.01 | -17.08 | -16.86 | -16.96 | -17.01 | -17.05 |
| $N_2$-5 | -15.06 | -15.36 | -15.51 | -15.64 | -15.31 | -15.46 | -15.51 | -15.54 |

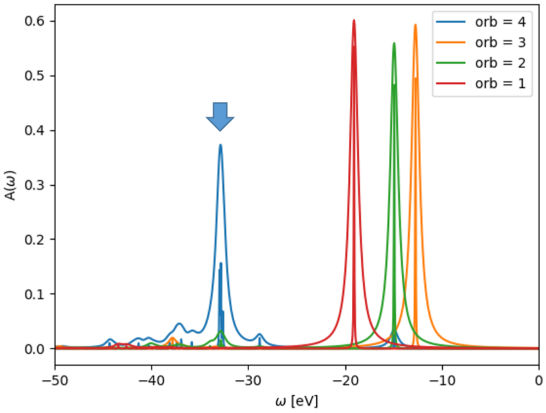


(a) $H_2O$. Resonance between ortbial 4 and 2.

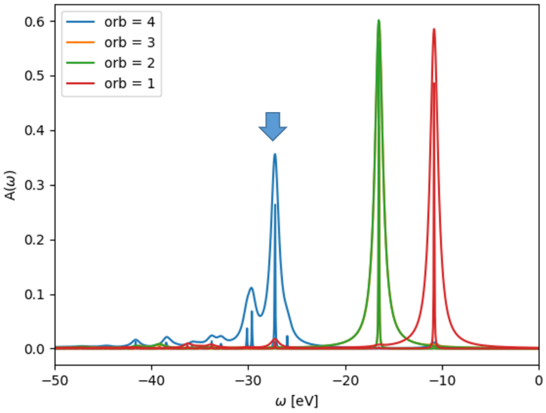


(b) $NH_3$. Resonance between orbital 4 and 1.

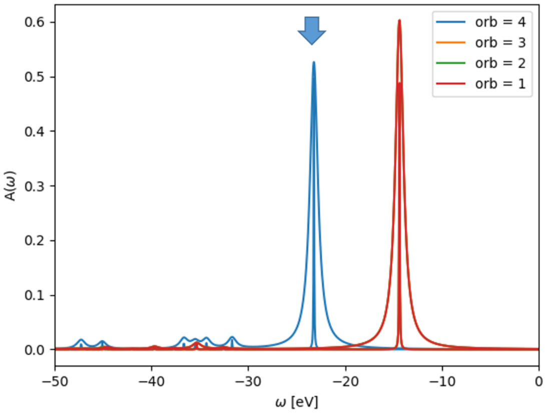


(c) $CH_4$. No appreciable resonance.

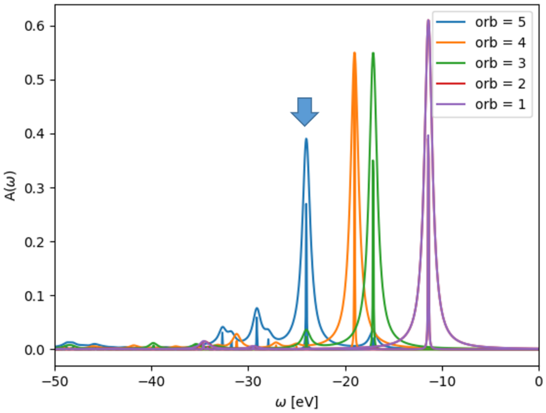


(d) $C_2H_2$. Resonance between orbital 5 and 3.

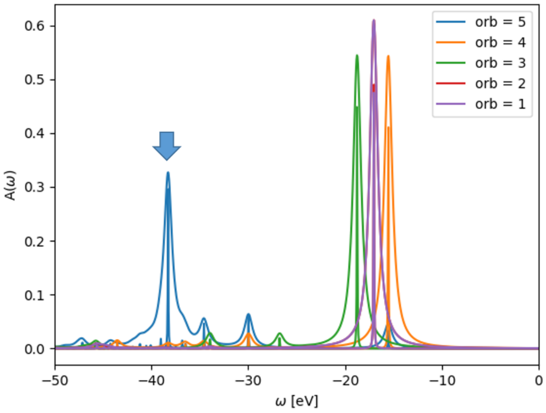


(e) $N_2$. Resonance between orbital 5 and 4.

Figure S3: Hole component of the spectral function for the molecules studied, orbital resolved, using the largest basis set. We use a broadening factor of $\sim 0.5$ eV. All molecules except for $CH_4$ show small resonances between the orbital furthest away from the HOMO (shown with an arrow) and another orbital.

## Quasiparticle energies and spectra for all methods

In Tab. S2 we summarize the quasiparticle energies obtained from all methods used in the paper (HF, $GW$, $GW\Gamma$ and ASCI) that are presented in Fig. (2) of the main paper. The ASCI results correspond to the values obtained by basis set extrapolation in the augmented basis set for all molecules except for $CH_4$, where the non-augmented basis set was used for the extrapolation. In Fig. S4 we show the spectral functions and self-energies for $H_2O$, $CH_4$, $C_2H_2$ and $N_2$.

**Table S2: QPE's of the valence orbitals for all molecules and the different methods presented in Fig. 2 in the main paper.**

| $H_2O$ | HF | $GW$ | $GW\Gamma$ | ASCI | $NH_3$ | HF | $GW$ | $GW\Gamma$ | ASCI |
|---|---|---|---|---|---|---|---|---|---|
| orb 1 | -36.82 | -35.06 | -32.02 | -32.99 | orb 1 | -31.08 | -29.22 | -27.58 | -27.36 |
| orb 2 | -19.51 | -19.62 | -19.20 | -19.10 | orb 2 | -17.12 | -17.11 | -16.70 | -16.51 |
| orb 3 | -15.92 | -15.44 | -15.03 | -14.90 | orb 3 | -17.12 | -17.11 | -16.70 | -16.51 |
| orb 4 | -13.88 | -13.36 | -12.94 | -12.75 | orb 4 | -11.70 | -11.69 | -10.85 | -10.81 |
| $CH_4$ | HF | $GW$ | $GW\Gamma$ | ASCI | | | | | |
| orb 1 | -25.69 | -24.21 | -22.74 | -23.25 | | | | | |
| orb 2 | -14.83 | -15.03 | -14.61 | -14.35 | | | | | |
| orb 3 | -14.83 | -15.03 | -14.61 | -14.35 | | | | | |
| orb 4 | -14.83 | -15.03 | -14.61 | -14.35 | | | | | |
| $C_2H_2$ | HF | $GW$ | $GW\Gamma$ | ASCI | $N_2$ | HF | $GW$ | $GW\Gamma$ | ASCI |
| orb 1 | -28.06 | -25.88 | -24.31 | -24.13 | orb 1 | -40.19 | -37.57 | -39.12 | -38.56 |
| orb 2 | -20.90 | -20.04 | -19.62 | -19.05 | orb 2 | -21.14 | -20.04 | -19.62 | -18.88 |
| orb 3 | -18.53 | -18.37 | -17.95 | -17.15 | orb 3 | -16.82 | -17.53 | -17.11 | -17.05 |
| orb 4 | -11.18 | -12.11 | -11.27 | -11.45 | orb 4 | -16.82 | -17.53 | -17.11 | -17.05 |
| orb 5 | -11.18 | -12.11 | -11.27 | -11.45 | orb 5 | -17.28 | -16.96 | -16.28 | -15.54 |

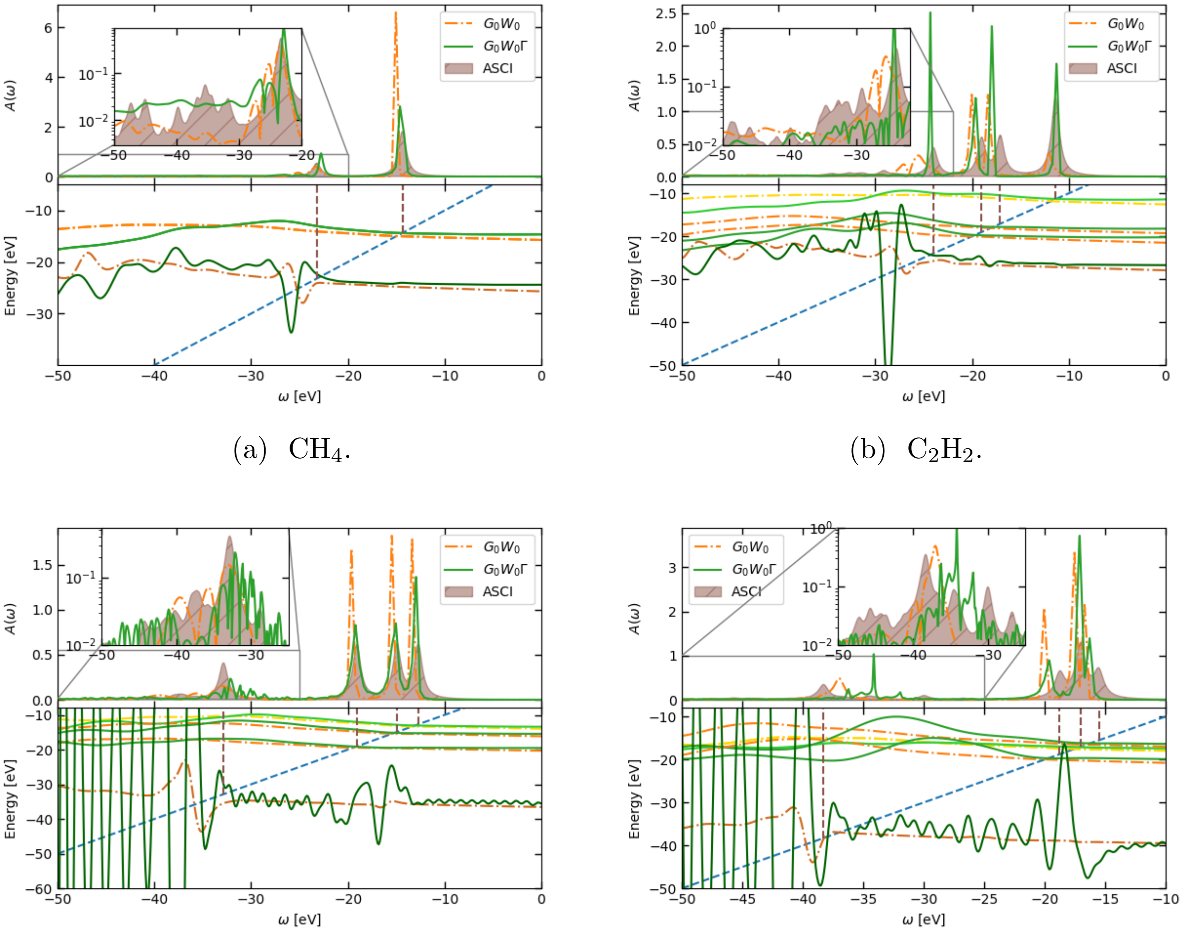


(a) $CH_4$.

(b) $C_2H_2$.

(c) $H_2O$.

(d) $N_2$.

Figure S4: Upper panels: Spectral functions for several molecules as computed with ASCI (filled curve), $G_0W_0$ (dot-dashed line) and $G_0W_0\Gamma$ (solid line). Lower panels: Corresponding real part of the diagonal self-energy terms, with graphical solution of the QP equation (2) of the main paper.

## Stochastic Many-body Perturbation Theory Calculations

The starting point calculations for the MBPT ground state calculations are performed with a real-space Hartree-Fock (HF) implementation. The formalism and implementations of the real-space and real-time stochastic many-body calculations are provided in Refs.[9,10] We employ Troullier-Martins pseudopotentials[11] and a kinetic energy cutoff of 28 $E_h$. The real-space grid parameters adopted in our calculations for each molecule are listed in Table S3.

**Table S3: Parameters of the HF calculations.**

| system | grid | grid spacing ($a_0$) |
|---|---|---|
| $H_2O$ | 72×60×70 | 0.30 |
| $NH_3$ | 66×66×60 | 0.30 |
| $CH_4$ | 72×72×72 | 0.30 |
| $C_2H_2$ | 72×72×90 | 0.30 |
| $N_2$ | 50×50×60 | 0.35 |

The quasipariticle energies are computed as

$$\varepsilon^{\mathrm{QP}} = \varepsilon^{\mathrm{HF}} + \left\langle \phi \middle| \hat{\Sigma}(\omega = \varepsilon^{\mathrm{QP}}) \middle| \phi \right\rangle \tag{4}$$

where $\varepsilon^{\mathrm{HF}}$ and $|\phi\rangle$ are the HF eigenvalue and the eigenstate. The $\Sigma$ is the self-energy term, yielding the electron correlation. Our MBPT calculations avoid the self-consistent renormalization.[12] Instead, we employ a one-shot correction on top of a HF starting point, whose single-electron orbitals are close to the true Dyson orbitals.[13] The Green's function in the HF basis is thus nearly diagonal (see the description of ASCI results). Most importantly, HF prevents the appearance of spurious MQP peaks in $GW$.[14–16] Note, however, that the one-shot treatment translates to an unscreened vertex term,[10,17,18] potentially overestimating the MQP couplings.

The self energies are computed via the one-shot $G_0W_0$ and the vertex-corrected $G_0W_0\Gamma$ method. In $G_0W_0$, the self-energy is expressed as

$$\Sigma(1,2) = i\nu(1,\bar{4})G(1,2)\nu(2,\bar{5})\chi(\bar{5},\bar{4}) \tag{5}$$

where $\chi(1,2)$ represents the two-point polarizability and $\nu$ the Coulomb kernel. The bar over the number means integrating over the space and time. In $G_0W_0\Gamma$, the expression reads

$$\Sigma(1,2) = i\nu(1,\bar{4})G(1,2)\nu(2,\bar{5})\chi(\bar{5},\bar{4}) - i\nu(1,\bar{4})G(1,\bar{3})\nu(\bar{3},2)^3\chi(\bar{3},2,\bar{4}) \tag{6}$$

Compared to $G_0W_0$, the extra term involving the three-point polarizability ${}^3\chi(1,2,3)$ in the

expression accounts for higher order electron correlation. See Refs.[10,19] for full discussion of the meaning of the higher order effects.

In the stochastic formalism, the Green's function is sampled by selecting random vectors $\zeta$, which sample the occupied and unoccupied subspace (propagated backward and forward in time). To make the expression for the self-energy separable, we use the sparse stochastic compression technique with additional set of sparse random vectors $\xi$.[9,20] The random vectors spanning the entire Hilbert space are constructed as $\pm \mathrm{d}V^{-1/2}$ (with uniform distribution on each real space grid point). Here, $\mathrm{d}V$ is the volume element of the grid. Occupied subspace sampling is achieved by projecting the random vectors on all occupied states of the underlying mean-field calculation.[9] The unoccupied subspace represents the complementary part of the random vector. For all systems we used a number of random vectors $N_\zeta = 1000$ and $N_\xi = 20000$. No other stochastic sampling is employed (unlike in calculations for large systems).

The real-time propagation limits the frequency resolution of the self-energy. In practice, we employ 50 a.u. maximum propagation time for excitations in the SQP regime. This value is consistent with our previous work for molecules and solids.[9,10,21,22] Resolution of the spectral features in the MQP regime requires (at least) three times larger propagation time (150 a.u.). Longer time evolution is subject to a large stochastic fluctuation and sampling bias. The longest simulations reported are thus based on the 150 a.u. propagation time. The convergence of the spectral features is illustrated in Fig. S5.

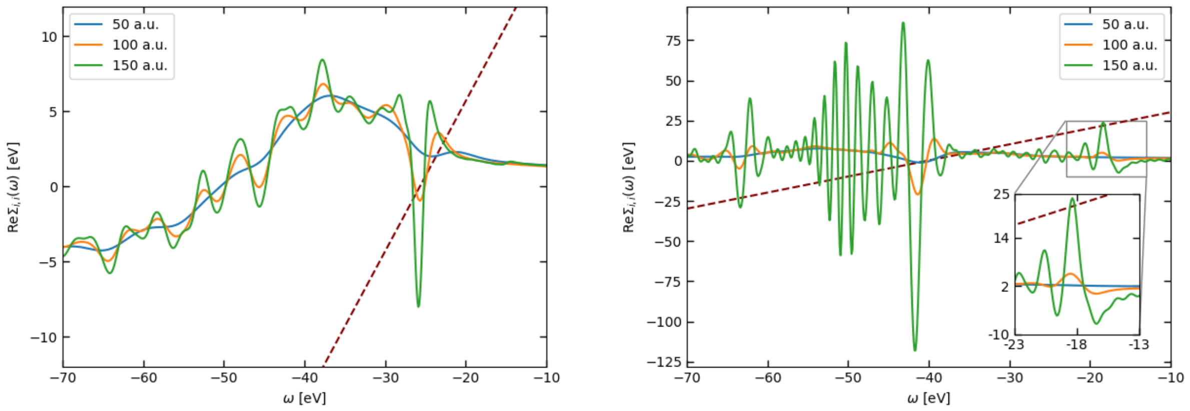


(a) $CH_4$.

(b) $N_2$.

Figure S5: Diagonal self energy components for the valence orbital furthest away from the HOMO for $N_2$ and $CH_4$ computed with vertex corrected $G_0W_0\Gamma$. Results are shown for different propagation times. The dashed line corresponds to the frequency line $y(\omega) = \omega$. See text for discussion.

# References


(1) Tubman, N. M.; Lee, J.; Takeshita, T. Y.; Head-Gordon, M.; Whaley, K. B. A deterministic alternative to the full configuration interaction quantum Monte Carlo method. *J. Chem. Phys.* **2016**, *145*, 044112.

(2) Tubman, N. M.; Mejuto-Zaera, C.; Epstein, J. M.; Hait, D.; Levine, D. S.; Huggins, W.; Jiang, Z.; McClean, J. R.; Babbush, R.; Head-Gordon, M. et al. Postponing the orthogonality catastrophe: efficient state preparation for electronic structure simulations on quantum devices. *ArXiv e-prints* **2018**,

(3) Tubman, N. M.; Freeman, C. D.; Levine, D. S.; Hait, D.; Head-Gordon, M.; Whaley, B. Modern Approaches to Exact Diagonalization and Selected Configuration Interaction with the Adaptive Sampling CI Method. *ArXiv e-prints* **2018**,

(4) Tubman, N. M.; Levine, D. S.; Hait, D.; Head-Gordon, M.; Whaley, K. B. An efficient

deterministic perturbation theory for selected configuration interaction methods. *arXiv preprint arXiv:1808.02049v1* **2018**,

(5) Mejuto-Zaera, C.; Tubman, N. M.; Whaley, K. B. Dynamical Mean-Field Theory Simulations with the Adaptive Sampling Configuration Interaction Method. *Phys. Rev. B* **2019**, *100*, 125165.

(6) Pavarini, E., Koch, E., Vollhardt, D., Lichtenstein, A., Eds. *The LDA+DMFT approach to strongly correlated materials*; Verlag des Forschungszentrum Jülich, 2011; Chapter 8, pp 235–264.

(7) Meyer, H. D.; Pal, S. A band-Lanczos method for computing matrix elements of a resolvent. *J. Chem. Phys.* **1989**, *91*, 6195.

(8) Rangel, T.; Hamed, S. M.; Bruneval, F.; Neaton, J. B. Evaluating the *GW* Approximation with CCSD(T) for Charged Excitations Across the Oligoacenes. *J. Chem. Theory Comput.* **2016**, *12*, 2834–2842.

(9) Vlček, V.; Li, W.; Baer, R.; Rabani, E.; Neuhauser, D. Swift *GW* beyond 10,000 electrons using sparse stochastic compression. *Phys. Rev. B* **2018**, *98*, 075107.

(10) Vlček, V. Stochastic Vertex Corrections: Linear Scaling Methods for Accurate Quasiparticle Energies. *J. Chem. Theory Comput.* **2019**, *15*, 6254.

(11) Troullier, N.; Martins, J. L. Efficient pseudopotentials for plane-wave calculations. *Phys. Rev. B* **1991**, *43*, 1993–2006.

(12) Hedin, L. New Method for Calculating the One-Particle Green's Function with Application to the Electron-Gas Problem. *Phys. Rev.* **1965**, *139*, A796–A823.

(13) Díaz-Tinoco, M.; Corzo, H. H.; Pawłowski, F.; Ortiz, J. V. Do Dyson Orbitals resemble canonical Hartree–Fock orbitals? *Mol. Phys.* **2019**, *117*, 2275.

(14) Véril, M.; Romaniello, P.; Berger, J. A.; Loos, P. Unphysical Discontinuities in *GW* methods. *J. Chem. Theory Comput.* **2018**, *14*, 5220.

(15) Golze, D.; Wilhelm, J.; van Setten, M. J.; Rinke, P. Core-Level Binding Energies from *GW*: An Efficient Full-Frequency Approach within a Localized Basis. *J. Chem. Theory Comput.* **2018**, *14*, 4856.

(16) Golze, D.; Keller, L.; Rinke, P. Accurate Absolute and Relative Core-Level Binding Energies from *GW*. *J. Phys. Chem. Lett.* **2020**, *11*, 1840.

(17) Romaniello, P.; Bechstedt, F.; Reining, L. Beyong *GW* approximation: Combining correlation channels. *Phys. Rev. B* **2012**, *85*, 155131.

(18) Maggio, E.; Kresse, G. GW Vertex Corrected Calculations for Molecular Systems. *J. Chem. Theory Comput.* **2017**, *13*, 4765.

(19) Martin, R. M.; Reining, L.; Ceperley, D. M. *Interacting Electrons: Theory and Computational Approaches*; Cambridge University Press, 2016.

(20) Neuhauser, D.; Gao, Y.; Arntsen, C.; Karshenas, C.; Rabani, E.; Baer, R. Breaking the Theoretical Scaling Limit for Predicting Quasiparticle energies: The Stochastic *GW* Approach. *Phys. Rev. Lett.* **2014**, *113*, 076402.

(21) Vlček, V.; Neuhauser, D.; Rabani, E.; Baer, R. Stochastic *GW* calculations for molecules. *J. Chem. Theory Comput.* **2017**, *13*, 4997.

(22) Vlček, V.; Rabani, E.; Neuhauser, D. Quasiparticle spectra from molecules to bulk. *Phys. Rev. Materials* **2018**, *2*, 030801(R).
